# Supplementary material for: Compact objects in modified gravity: junction conditions and other viability criteria
Source: arXiv:2312.03757 source file (2023-12-04)
Supplement: Supplementary file 1 [file AppendixTablesBSPGT.tex]

\chapter{Singular contributions to the equations of motion of \BSPGT.}
\label{app:tablesterms}
In the first column of the following tables, we show the different types of terms as they appear in the equations of motion (with $t^\rho{}_{\mu\nu}=0$) \eqref{eq:EoM1}-\eqref{eq:EoM3}. In the second column, we present the terms arising from the aforementioned terms in the first column when expressed in terms of basic variables and their derivatives (including Levi-Civita curvatures). Then, in the third column, we show both the regular and singular contributions obtained from the previous terms when promoted to distributions while subject to the preliminary conditions \eqref{eq:condNoSingTSg}-\eqref{eq:condnojumpg}. Finally, in the last column we display the  terms that survive the enforcement of all the consistency conditions \eqref{eq:condNoSingTSg}-\eqref{eq:condJumpnS}. Indices of the vectors have been omitted for clarity almost everywhere in the following tables, except for the combination $\alpha\LCD_\mu S^\mu$, in order to clearly signal where condition \eqref{eq:condJumpnS} has been used. Finally, we clarify that by ``undefined as distribution'' we mean that those terms would contain powers of singular parts. Recall that, although the products of $\udis{\Theta}\,\udis{\Theta}$ and $\udis{\Theta}\del$ would also be mathematically undefined, our prescription \eqref{eq:prescTheDel} allows to deal with them. 

\begin{table}[h!]
    \centering
    
    \begin{tabular}{ m{2.5cm} m{3.5cm} m{3.5cm} m{3.5cm} }
    \hline
    {\footnotesize Terms in \eqref{eq:EoM1}} & {\footnotesize In terms of basic fields} & {\footnotesize Pieces after \eqref{eq:condNoSingTSg}--\eqref{eq:condnojumpg}} & {\footnotesize Pieces after \eqref{eq:condNoSingTSg}--\eqref{eq:condJumpnS}}\\
    \hline
    \hline
    $M_T^2 T$&  $M_T^2 T$     & $\varrho$  & $\varrho$  \\ 
    \hline
    \multirow{3}{*}{$\beta T \MAR $} 
    &$\beta T \LCR$           & $\varrho + \Delta^{\szero}$  & $\varrho$ \\ 
    &$\beta T \LCD T$         & $\varrho + \Delta^{\szero}$  & $\varrho$ \\ 
    &$\beta SST, \beta TTT$   & $\varrho$                 & $\varrho$ (continuous) \\
    \hline
    \multirow{2}{*}{$\alpha S\mathcal{H} $}
    &$\alpha S\LCD_\mu S^\mu$ & $\varrho + \Delta^{\szero}$  & $\varrho$ \\ 
    &$\alpha TSS$             & $\varrho $                & $\varrho$ \\ 
    \hline
    \multirow{3}{*}{$\beta \LCD R$} 
    &$\beta \LCD \LCR$        & $\varrho + \Delta^{\szero}+ \Delta^{\sone}$  & $\varrho+ \Delta^{\szero}$ \\ 
    &$\beta \LCD \LCD T$      & $\varrho + \Delta^{\szero}+ \Delta^{\sone}$  & $\varrho+ \Delta^{\szero}$ \\ 
    &$\beta S\LCD S$, $\beta T\LCD T$          & $\varrho + \Delta^{\szero}$  & $\varrho$ \\
    \hline
    \hline
\end{tabular}
    
    \caption[Terms in the equation of $T_\mu$ in \BSPGT, and their respective regular and singular parts after distributional promotion.]{Terms in the equation of $T_\mu$, \eqref{eq:EoM1}, and their respective regular and singular parts after distributional promotion.}
\end{table}

\begin{table}[h!]
    \centering
    
    \begin{tabular}{ m{2.5cm} m{3.5cm} m{3.5cm} m{3.5cm} } 
    \hline
    {\footnotesize Terms in \eqref{eq:EoM2}} & {\footnotesize In terms of basic fields} & {\footnotesize Pieces after \eqref{eq:condNoSingTSg}--\eqref{eq:condnojumpg}} & {\footnotesize Pieces after \eqref{eq:condNoSingTSg}--\eqref{eq:condJumpnS}}\\
    \hline
    \hline
    $M_S^2 S$&  $M_S^2 S$       & $\varrho$  & $\varrho$  \\ 
    \hline
    \multirow{3}{*}{$\beta S \MAR $} 
    &$\beta S \LCR$             & $\varrho + \Delta^{\szero}$  & $\varrho$ \\ 
    &$\beta S \LCD T$           & $\varrho + \Delta^{\szero}$  & $\varrho$ \\ 
    &$\beta SSS, \beta STT$     & $\varrho$                 & $\varrho$ (continuous) \\
    \hline
    \multirow{2}{*}{$\alpha T\mathcal{H}$}
    &$\alpha T\LCD_\mu S^\mu$   & $\varrho + \Delta^{\szero}$  & $\varrho$ \\ 
    &$\alpha STT$               & $\varrho $                & $\varrho$ \\ 
    \hline
    \multirow{2}{*}{$\alpha \LCD \mathcal{H}$} 
    &$\alpha\LCD(\LCD_\mu S^\mu)$ & $\varrho + \Delta^{\szero}+ \Delta^{\sone}$  & $\varrho+ \Delta^{\szero}$ \\ 
    &$\alpha T\LCD S$, $\alpha S\LCD T$           & $\varrho + \Delta^{\szero}$  & $\varrho + \Delta^{\szero}$ \\
    \hline
    \hline
\end{tabular}
    
    \caption[Terms in the equation of $S_\mu$ in \BSPGT, and their respective regular and singular parts after distributional promotion.]{Terms in the equation of $S_\mu$, \eqref{eq:EoM2}, and their respective regular and singular parts after distributional promotion.}
\end{table}

\begin{table}[h!]
    \centering
    
    \begin{tabular}{ m{2.5cm} m{3.5cm} m{3.5cm} m{3.5cm} } 
    \hline
    {\footnotesize Terms in \eqref{eq:EoM3}} & {\footnotesize In terms of basic fields} & {\footnotesize Pieces after \eqref{eq:condNoSingTSg}--\eqref{eq:condnojumpg}} & {\footnotesize Pieces after \eqref{eq:condNoSingTSg}--\eqref{eq:condJumpnS}}\\
    \hline
    \hline
    $M_S^2 SS$, $M_T^2 TT$&  $M_S^2 SS$, $M_T^2 TT$& $\varrho$  & $\varrho$  \\ 
    \hline
    $\Mp^2\LCR_{\mu\nu}$&  $\Mp^2\LCR_{\mu\nu}$& $\varrho+ \Delta^{\szero}$  & $\varrho+ \Delta^{\szero}$  \\ 
    \hline
    \multirow{3}{*}{$\beta\LCR_{\mu\nu}\MAR$} 
    &$\beta\LCR_{\mu\nu}\LCR$     & distrib.~undefined  & $\varrho+ \Delta^{\szero}$ \\ 
    &$\beta\LCR_{\mu\nu} \LCD T$  & distrib.~undefined  & $\varrho$ \\ 
    &$\beta\LCR_{\mu\nu} TT$, $\beta\LCR_{\mu\nu} SS$   & $\varrho+ \Delta^{\szero}$                 & $\varrho+ \Delta^{\szero}$ \\
    \hline
    \multirow{3}{*}{$\beta TT \MAR $} 
    &$\beta TT \LCR$           & $\varrho + \Delta^{\szero}$  & $\varrho$ \\ 
    &$\beta TT \LCD T$         & $\varrho + \Delta^{\szero}$  & $\varrho$ \\ 
    &$\beta SSTT, \beta TTTT$   & $\varrho$                 & $\varrho$ (continuous) \\
    \hline
    \multirow{3}{*}{$\beta SS \MAR $} 
    &$\beta SS \LCR$           & $\varrho + \Delta^{\szero}$  & $\varrho$ \\ 
    &$\beta SS \LCD T$         & $\varrho + \Delta^{\szero}$  & $\varrho$ \\ 
    &$\beta SSSS, \beta SSTT$   & $\varrho$                 & $\varrho$ (continuous) \\ 
    \hline
    \multirow{2}{*}{$\alpha TS\mathcal{H} $}
    &$\alpha TS\LCD_\mu S^\mu$ & $\varrho + \Delta^{\szero}$  & $\varrho$ \\ 
    &$\alpha TTSS$             & $\varrho $                & $\varrho$ \\  
    \hline
    \multirow{3}{*}{$\beta T\LCD \MAR$} 
    &$\beta T \LCD \LCR$        & $\varrho + \Delta^{\szero}+ \Delta^{\sone}$  & $\varrho+ \Delta^{\szero}$ \\ 
    &$\beta T \LCD \LCD T$      & $\varrho + \Delta^{\szero}+ \Delta^{\sone}$  & $\varrho+ \Delta^{\szero}$ \\ 
    &$\beta TS\LCD S$, $\beta TT\LCD T$          & $\varrho + \Delta^{\szero}$  & $\varrho$ \\
    \hline
    \multirow{2}{*}{$\alpha S \LCD \mathcal{H}$} 
    &$\alpha S\LCD(\LCD_\mu S^\mu)$ & $\varrho + \Delta^{\szero}+ \Delta^{\sone}$  & $\varrho+ \Delta^{\szero}$ \\ 
    &$\alpha TS\LCD S$, $\alpha SS\LCD T$           & $\varrho + \Delta^{\szero}$  & $\varrho + \Delta^{\szero}$ \\ 
    \hline
    \multirow{3}{*}{$\alpha \mathcal{H}^2$} 
    &$\alpha(\LCD_\mu S^\mu)^2$ & distrib.~undefined  & $\varrho$ \\ 
    &$\alpha ST\LCD_\mu S^\mu$  & $\varrho + \Delta^{\szero}$  & $\varrho$ \\
    &$\alpha SSTT$              & $\varrho$  & $\varrho$ \\
    \hline
    \multirow{6}{*}{$\beta \MAR^2$} 
    &$\beta \LCR^2$                   & distrib.~undefined  & $\varrho$ \\ 
    &$\beta \LCR\LCD T$               & distrib.~undefined  & $\varrho$ \\ 
    &$\beta SS\LCR$, $\beta TT\LCR$    & $\varrho + \Delta^{\szero}$  & $\varrho$ \\ 
    &$\beta \LCD T \LCD T$            & distrib.~undefined  & $\varrho$ \\ 
    &$\beta SS\LCD T$, $\beta TT\LCD T$& $\varrho + \Delta^{\szero}$  & $\varrho$ \\ 
    &$\beta \times \text{(powers of}\,T,S\text{)}$ &$\varrho$  & $\varrho$ (continuous) \\
    \hline
    \multirow{4}{*}{$\beta \LCD\LCD \MAR$} 
    &$\beta \LCD\LCD \LCR$                   & $\varrho + \Delta^{\szero}+ \Delta^{\sone}+ \Delta^{\stwo}$ & $\varrho + \Delta^{\szero}+ \Delta^{\sone}$ \\ 
    &$\beta \LCD\LCD\LCD T$               & $\varrho + \Delta^{\szero}+ \Delta^{\sone}+ \Delta^{\stwo}$ & $\varrho + \Delta^{\szero}+ \Delta^{\sone}$ \\ 
    &$\beta S\LCD\LCD S$, $\beta T \LCD\LCD T$    & $\varrho + \Delta^{\szero}+ \Delta^{\sone}$  & $\varrho+ \Delta^{\szero}$ \\ 
    &$\beta \LCD T \LCD T$, $\beta \LCD S \LCD S$            & distrib.~undefined  & $\varrho$ \\ 
    \hline
    \hline
\end{tabular}
    
    \caption[Terms in the equation of $g_{\mu\nu}$ in \BSPGT, and their respective regular and singular parts after distributional promotion.]{Terms in the equation of $g_{\mu\nu}$, \eqref{eq:EoM3}, and their respective regular and singular parts after distributional promotion.}
\end{table}
